# Supplementary material for: Electric dipole polarizabilities of Rydberg states of alkali atoms
Source: arXiv:1608.04515 source file (2016-08-16)
Supplement: Supplementary file 1 [file poldf15_suppl.pdf]

# Electric dipole polarizabilities of Rydberg states of alkali atoms – Supplementary material

V. A. Yerokhin,[1,2] S. Y. Buhmann,[3,4] S. Fritzsche,[5,6] and A. Surzhykov[1,7]

[1]*Physikalisch-Technische Bundesanstalt, D-38116 Braunschweig, Germany*
[2]*Center for Advanced Studies, Peter the Great St. Petersburg Polytechnic University, 195251 St. Petersburg, Russia*
[3]*Physikalisches Institut, Albert-Ludwigs Univesität Freiburg, D-79104 Freiburg, Germany*
[4]*Freiburg Institute for Advanced Studies, Albert-Ludwigs Universität Freiburg, D-79104 Freiburg, Germany*
[5]*Helmholtz-Institut Jena, D-07743 Jena, Germany*
[6]*Theoretisch-Physikalisches Institut, Friedrich-Schiller-Universität Jena, D-07743 Jena, Germany*
[7]*Technische Univesität Braunschweig, D-38106 Braunschweig, Germany*

In this Supplementary Material we present tabulations of our numerical results obtained by the Dirac-Fock Core-Polarization (DFCP) method for the static electric-dipole scalar and tensor polarizabilities $\alpha_0$ and $\alpha_2$ for the $nS$, $nP_{1/2,\,3/2}$, and $nD_{3/2,\,5/2}$ states of two alkali atoms, Rb and Cs. The corresponding numerical values are listed in Tables I-IV. Results are reported for the states with the principal quantum number $n = 8-50$ for Rb and $n = 9-50$ for Cs.

TABLE I: Static electric-dipole scalar polarizabilities $\alpha_0$ for Rb, in $a_0^3$ ($a_0 \approx 0.052\,918$ nm is the Bohr radius). $X[b]$ means $X \times 10^b$.

| $n$ | $n^2S$ | $n^2P_{1/2}$ | $n^2P_{3/2}$ | $n^2D_{3/2}$ | $n^2D_{5/2}$ |
|---|---|---|---|---|---|
| 8 | 0.133 [6] | 0.363 [6] | 0.395 [6] | 0.909 [6] | 0.877 [6] |
| 9 | 0.417 [6] | 0.120 [7] | 0.130 [7] | 0.221 [7] | 0.212 [7] |
| 10 | 0.109 [7] | 0.328 [7] | 0.357 [7] | 0.479 [7] | 0.458 [7] |
| 11 | 0.252 [7] | 0.787 [7] | 0.859 [7] | 0.956 [7] | 0.909 [7] |
| 12 | 0.528 [7] | 0.171 [8] | 0.187 [8] | 0.178 [8] | 0.169 [8] |
| 13 | 0.102 [8] | 0.343 [8] | 0.375 [8] | 0.314 [8] | 0.296 [8] |
| 14 | 0.186 [8] | 0.644 [8] | 0.706 [8] | 0.530 [8] | 0.498 [8] |
| 15 | 0.321 [8] | 0.115 [9] | 0.126 [9] | 0.858 [8] | 0.803 [8] |
| 16 | 0.531 [8] | 0.196 [9] | 0.215 [9] | 0.135 [9] | 0.126 [9] |
| 17 | 0.847 [8] | 0.321 [9] | 0.352 [9] | 0.205 [9] | 0.191 [9] |
| 18 | 0.131 [9] | 0.509 [9] | 0.559 [9] | 0.304 [9] | 0.282 [9] |
| 19 | 0.197 [9] | 0.784 [9] | 0.862 [9] | 0.442 [9] | 0.408 [9] |
| 20 | 0.289 [9] | 0.118 [10] | 0.130 [10] | 0.629 [9] | 0.580 [9] |
| 21 | 0.416 [9] | 0.173 [10] | 0.191 [10] | 0.880 [9] | 0.808 [9] |
| 22 | 0.586 [9] | 0.249 [10] | 0.274 [10] | 0.121 [10] | 0.111 [10] |
| 23 | 0.813 [9] | 0.352 [10] | 0.388 [10] | 0.164 [10] | 0.150 [10] |
| 24 | 0.111 [10] | 0.489 [10] | 0.540 [10] | 0.220 [10] | 0.200 [10] |
| 25 | 0.149 [10] | 0.670 [10] | 0.740 [10] | 0.291 [10] | 0.264 [10] |
| 26 | 0.198 [10] | 0.906 [10] | 1.000 [10] | 0.380 [10] | 0.345 [10] |
| 27 | 0.260 [10] | 0.121 [11] | 0.133 [11] | 0.492 [10] | 0.445 [10] |
| 28 | 0.338 [10] | 0.159 [11] | 0.176 [11] | 0.630 [10] | 0.570 [10] |
| 29 | 0.435 [10] | 0.208 [11] | 0.230 [11] | 0.801 [10] | 0.722 [10] |
| 30 | 0.555 [10] | 0.269 [11] | 0.297 [11] | 0.101 [11] | 0.909 [10] |
| 31 | 0.701 [10] | 0.344 [11] | 0.381 [11] | 0.126 [11] | 0.113 [11] |
| 32 | 0.879 [10] | 0.437 [11] | 0.484 [11] | 0.157 [11] | 0.141 [11] |
| 33 | 0.109 [11] | 0.551 [11] | 0.610 [11] | 0.193 [11] | 0.173 [11] |
| 34 | 0.135 [11] | 0.689 [11] | 0.763 [11] | 0.237 [11] | 0.212 [11] |
| 35 | 0.166 [11] | 0.856 [11] | 0.948 [11] | 0.289 [11] | 0.258 [11] |
| 36 | 0.202 [11] | 0.106 [12] | 0.117 [12] | 0.350 [11] | 0.312 [11] |
| 37 | 0.246 [11] | 0.130 [12] | 0.143 [12] | 0.422 [11] | 0.375 [11] |
| 38 | 0.296 [11] | 0.158 [12] | 0.175 [12] | 0.506 [11] | 0.450 [11] |
| 39 | 0.356 [11] | 0.191 [12] | 0.212 [12] | 0.604 [11] | 0.536 [11] |
| 40 | 0.425 [11] | 0.231 [12] | 0.256 [12] | 0.718 [11] | 0.636 [11] |
| 41 | 0.506 [11] | 0.277 [12] | 0.307 [12] | 0.850 [11] | 0.752 [11] |
| 42 | 0.599 [11] | 0.331 [12] | 0.367 [12] | 0.100 [12] | 0.885 [11] |
| 43 | 0.707 [11] | 0.394 [12] | 0.437 [12] | 0.118 [12] | 0.104 [12] |
| 44 | 0.830 [11] | 0.467 [12] | 0.518 [12] | 0.138 [12] | 0.121 [12] |
| 45 | 0.972 [11] | 0.551 [12] | 0.611 [12] | 0.160 [12] | 0.141 [12] |
| 46 | 0.113 [12] | 0.647 [12] | 0.718 [12] | 0.186 [12] | 0.164 [12] |
| 47 | 0.132 [12] | 0.758 [12] | 0.841 [12] | 0.216 [12] | 0.189 [12] |
| 48 | 0.153 [12] | 0.884 [12] | 0.981 [12] | 0.249 [12] | 0.219 [12] |
| 49 | 0.176 [12] | 0.103 [13] | 0.114 [13] | 0.287 [12] | 0.251 [12] |
| 50 | 0.203 [12] | 0.119 [13] | 0.132 [13] | 0.329 [12] | 0.288 [12] |

TABLE II: Static electric-dipole tensor polarizabilities $\alpha_2$ for Rb, in $a_0^5$. Notations are as in Table I.

| $n$ | $n^2P_{3/2}$ | $n^2D_{3/2}$ | $n^2D_{5/2}$ |
|---|---|---|---|
| 8 | −0.513 [5] | 0.113 [6] | 0.223 [6] |
| 9 | −0.161 [6] | 0.389 [6] | 0.723 [6] |
| 10 | −0.427 [6] | 0.107 [7] | 0.194 [7] |
| 11 | −0.996 [6] | 0.256 [7] | 0.455 [7] |
| 12 | −0.211 [7] | 0.552 [7] | 0.968 [7] |
| 13 | −0.414 [7] | 0.110 [8] | 0.191 [8] |
| 14 | −0.765 [7] | 0.204 [8] | 0.353 [8] |
| 15 | −0.134 [8] | 0.361 [8] | 0.620 [8] |
| 16 | −0.225 [8] | 0.611 [8] | 0.104 [9] |
| 17 | −0.364 [8] | 0.994 [8] | 0.169 [9] |
| 18 | −0.571 [8] | 0.157 [9] | 0.266 [9] |
| 19 | −0.871 [8] | 0.240 [9] | 0.406 [9] |
| 20 | −0.130 [9] | 0.359 [9] | 0.606 [9] |
| 21 | −0.189 [9] | 0.524 [9] | 0.884 [9] |
| 22 | −0.269 [9] | 0.751 [9] | 0.126 [10] |
| 23 | −0.378 [9] | 0.106 [10] | 0.178 [10] |
| 24 | −0.521 [9] | 0.146 [10] | 0.246 [10] |
| 25 | −0.710 [9] | 0.200 [10] | 0.335 [10] |
| 26 | −0.953 [9] | 0.269 [10] | 0.451 [10] |
| 27 | −0.126 [10] | 0.358 [10] | 0.600 [10] |
| 28 | −0.166 [10] | 0.471 [10] | 0.788 [10] |
| 29 | −0.215 [10] | 0.614 [10] | 0.103 [11] |
| 30 | −0.277 [10] | 0.791 [10] | 0.132 [11] |
| 31 | −0.353 [10] | 0.101 [11] | 0.169 [11] |
| 32 | −0.447 [10] | 0.128 [11] | 0.214 [11] |
| 33 | −0.561 [10] | 0.161 [11] | 0.268 [11] |
| 34 | −0.699 [10] | 0.201 [11] | 0.335 [11] |
| 35 | −0.865 [10] | 0.249 [11] | 0.415 [11] |
| 36 | −0.106 [11] | 0.307 [11] | 0.511 [11] |
| 37 | −0.130 [11] | 0.376 [11] | 0.626 [11] |
| 38 | −0.158 [11] | 0.458 [11] | 0.761 [11] |
| 39 | −0.191 [11] | 0.554 [11] | 0.921 [11] |
| 40 | −0.230 [11] | 0.668 [11] | 0.111 [12] |
| 41 | −0.275 [11] | 0.801 [11] | 0.133 [12] |
| 42 | −0.328 [11] | 0.955 [11] | 0.159 [12] |
| 43 | −0.389 [11] | 0.114 [12] | 0.188 [12] |
| 44 | −0.460 [11] | 0.134 [12] | 0.223 [12] |
| 45 | −0.541 [11] | 0.158 [12] | 0.263 [12] |
| 46 | −0.634 [11] | 0.186 [12] | 0.308 [12] |
| 47 | −0.741 [11] | 0.217 [12] | 0.361 [12] |
| 48 | −0.863 [11] | 0.254 [12] | 0.420 [12] |
| 49 | −0.100 [12] | 0.295 [12] | 0.488 [12] |
| 50 | −0.116 [12] | 0.341 [12] | 0.566 [12] |

TABLE III: Static electric-dipole scalar polarizabilities $\alpha_0$ for Cs, in $a_0^3$.

| $n$ | $n^2S$ | $n^2P_{1/2}$ | $n^2P_{3/2}$ | $n^2D_{3/2}$ | $n^2D_{5/2}$ |
|---|---|---|---|---|---|
| 9 | 0.154 [6] | 0.105 [7] | 0.136 [7] | −0.146 [7] | −0.185 [7] |
| 10 | 0.477 [6] | 0.356 [7] | 0.463 [7] | −0.436 [7] | −0.548 [7] |
| 11 | 0.125 [7] | 0.100 [8] | 0.131 [8] | −0.111 [8] | −0.139 [8] |
| 12 | 0.286 [7] | 0.246 [8] | 0.321 [8] | −0.254 [8] | −0.315 [8] |
| 13 | 0.598 [7] | 0.543 [8] | 0.709 [8] | −0.530 [8] | −0.655 [8] |
| 14 | 0.116 [8] | 0.110 [9] | 0.144 [9] | −0.103 [9] | −0.127 [9] |
| 15 | 0.211 [8] | 0.210 [9] | 0.275 [9] | −0.188 [9] | −0.231 [9] |
| 16 | 0.365 [8] | 0.378 [9] | 0.496 [9] | −0.328 [9] | −0.403 [9] |
| 17 | 0.605 [8] | 0.651 [9] | 0.853 [9] | −0.550 [9] | −0.672 [9] |
| 18 | 0.967 [8] | 0.108 [10] | 0.141 [10] | −0.887 [9] | −0.108 [10] |
| 19 | 0.150 [9] | 0.172 [10] | 0.226 [10] | −0.139 [10] | −0.169 [10] |
| 20 | 0.226 [9] | 0.267 [10] | 0.350 [10] | −0.212 [10] | −0.258 [10] |
| 21 | 0.332 [9] | 0.403 [10] | 0.529 [10] | −0.315 [10] | −0.383 [10] |
| 22 | 0.479 [9] | 0.596 [10] | 0.782 [10] | −0.458 [10] | −0.557 [10] |
| 23 | 0.677 [9] | 0.862 [10] | 0.113 [11] | −0.654 [10] | −0.794 [10] |
| 24 | 0.941 [9] | 0.122 [11] | 0.161 [11] | −0.918 [10] | −0.111 [11] |
| 25 | 0.129 [10] | 0.171 [11] | 0.224 [11] | −0.127 [11] | −0.154 [11] |
| 26 | 0.174 [10] | 0.235 [11] | 0.309 [11] | −0.173 [11] | −0.209 [11] |
| 27 | 0.231 [10] | 0.319 [11] | 0.419 [11] | −0.232 [11] | −0.281 [11] |
| 28 | 0.304 [10] | 0.427 [11] | 0.561 [11] | −0.308 [11] | −0.373 [11] |
| 29 | 0.397 [10] | 0.565 [11] | 0.742 [11] | −0.405 [11] | −0.490 [11] |
| 30 | 0.511 [10] | 0.740 [11] | 0.972 [11] | −0.526 [11] | −0.636 [11] |
| 31 | 0.653 [10] | 0.959 [11] | 0.126 [12] | −0.678 [11] | −0.819 [11] |
| 32 | 0.827 [10] | 0.123 [12] | 0.162 [12] | −0.865 [11] | −0.104 [12] |
| 33 | 0.104 [11] | 0.157 [12] | 0.206 [12] | −0.110 [12] | −0.132 [12] |
| 34 | 0.130 [11] | 0.198 [12] | 0.260 [12] | −0.138 [12] | −0.166 [12] |
| 35 | 0.160 [11] | 0.248 [12] | 0.326 [12] | −0.172 [12] | −0.207 [12] |
| 36 | 0.197 [11] | 0.309 [12] | 0.406 [12] | −0.213 [12] | −0.256 [12] |
| 37 | 0.241 [11] | 0.382 [12] | 0.502 [12] | −0.262 [12] | −0.315 [12] |
| 38 | 0.294 [11] | 0.469 [12] | 0.616 [12] | −0.320 [12] | −0.386 [12] |
| 39 | 0.355 [11] | 0.573 [12] | 0.753 [12] | −0.390 [12] | −0.469 [12] |
| 40 | 0.427 [11] | 0.696 [12] | 0.914 [12] | −0.471 [12] | −0.567 [12] |
| 41 | 0.511 [11] | 0.841 [12] | 0.110 [13] | −0.568 [12] | −0.683 [12] |
| 42 | 0.609 [11] | 0.101 [13] | 0.133 [13] | −0.680 [12] | −0.818 [12] |
| 43 | 0.723 [11] | 0.121 [13] | 0.159 [13] | −0.811 [12] | −0.976 [12] |
| 44 | 0.854 [11] | 0.144 [13] | 0.189 [13] | −0.963 [12] | −0.116 [13] |
| 45 | 0.100 [12] | 0.171 [13] | 0.225 [13] | −0.114 [13] | −0.137 [13] |
| 46 | 0.118 [12] | 0.202 [13] | 0.265 [13] | −0.134 [13] | −0.161 [13] |
| 47 | 0.138 [12] | 0.237 [13] | 0.312 [13] | −0.158 [13] | −0.189 [13] |
| 48 | 0.160 [12] | 0.278 [13] | 0.366 [13] | −0.184 [13] | −0.221 [13] |
| 49 | 0.186 [12] | 0.325 [13] | 0.428 [13] | −0.215 [13] | −0.258 [13] |
| 50 | 0.215 [12] | 0.379 [13] | 0.498 [13] | −0.249 [13] | −0.300 [13] |

TABLE IV: Static electric-dipole tensor polarizabilities $\alpha_2$ for Cs, in $a_0^5$.

| $n$ | $n^2P_{3/2}$ | $n^2D_{3/2}$ | $n^2D_{5/2}$ |
|---|---|---|---|
| 9 | −0.138 [6] | 0.121 [7] | 0.245 [7] |
| 10 | −0.460 [6] | 0.347 [7] | 0.701 [7] |
| 11 | −0.127 [7] | 0.860 [7] | 0.174 [8] |
| 12 | −0.308 [7] | 0.192 [8] | 0.387 [8] |
| 13 | −0.673 [7] | 0.393 [8] | 0.792 [8] |
| 14 | −0.136 [8] | 0.753 [8] | 0.152 [9] |
| 15 | −0.257 [8] | 0.136 [9] | 0.274 [9] |
| 16 | −0.460 [8] | 0.235 [9] | 0.474 [9] |
| 17 | −0.786 [8] | 0.391 [9] | 0.786 [9] |
| 18 | −0.129 [9] | 0.627 [9] | 0.126 [10] |
| 19 | −0.206 [9] | 0.975 [9] | 0.196 [10] |
| 20 | −0.319 [9] | 0.148 [10] | 0.297 [10] |
| 21 | −0.480 [9] | 0.219 [10] | 0.439 [10] |
| 22 | −0.707 [9] | 0.317 [10] | 0.637 [10] |
| 23 | −0.102 [10] | 0.451 [10] | 0.905 [10] |
| 24 | −0.145 [10] | 0.631 [10] | 0.127 [11] |
| 25 | −0.202 [10] | 0.870 [10] | 0.174 [11] |
| 26 | −0.277 [10] | 0.118 [11] | 0.237 [11] |
| 27 | −0.375 [10] | 0.158 [11] | 0.317 [11] |
| 28 | −0.501 [10] | 0.210 [11] | 0.420 [11] |
| 29 | −0.662 [10] | 0.275 [11] | 0.551 [11] |
| 30 | −0.865 [10] | 0.357 [11] | 0.714 [11] |
| 31 | −0.112 [11] | 0.459 [11] | 0.918 [11] |
| 32 | −0.144 [11] | 0.585 [11] | 0.117 [12] |
| 33 | −0.183 [11] | 0.739 [11] | 0.148 [12] |
| 34 | −0.230 [11] | 0.927 [11] | 0.185 [12] |
| 35 | −0.288 [11] | 0.115 [12] | 0.231 [12] |
| 36 | −0.359 [11] | 0.143 [12] | 0.286 [12] |
| 37 | −0.443 [11] | 0.176 [12] | 0.351 [12] |
| 38 | −0.544 [11] | 0.215 [12] | 0.429 [12] |
| 39 | −0.664 [11] | 0.261 [12] | 0.521 [12] |
| 40 | −0.806 [11] | 0.315 [12] | 0.630 [12] |
| 41 | −0.973 [11] | 0.379 [12] | 0.758 [12] |
| 42 | −0.117 [12] | 0.454 [12] | 0.907 [12] |
| 43 | −0.140 [12] | 0.541 [12] | 0.108 [13] |
| 44 | −0.166 [12] | 0.642 [12] | 0.128 [13] |
| 45 | −0.197 [12] | 0.759 [12] | 0.152 [13] |
| 46 | −0.233 [12] | 0.893 [12] | 0.178 [13] |
| 47 | −0.274 [12] | 0.105 [13] | 0.209 [13] |
| 48 | −0.321 [12] | 0.122 [13] | 0.245 [13] |
| 49 | −0.375 [12] | 0.143 [13] | 0.285 [13] |
| 50 | −0.436 [12] | 0.166 [13] | 0.331 [13] |
